# Supplementary material for: CitySTAR: Structured and Topology-Aware Reasoning for Open-Vocabulary Urban 3D Grounding
Source: arXiv:2609.19911 source file (2026-11-09)
Supplement: Supplementary file 1 [file appendix.tex]

\section{Supplementary Material}



\subsection{Agentic Implementation Details of CitySTAR}
\label{app:agentic_details}

\begin{figure}[h]
    \centering
    \includegraphics[width=1\linewidth]{Figs/CitySTAR.png}
    \caption{Agent-based implementation view of CitySTAR. The main paper presents CitySTAR as a structured three-stage pipeline, while this supplementary figure illustrates how the pipeline is realized through collaborative functional agents for scene construction, query analysis, tool orchestration, topology verification, and reflective cross-modal grounding.}
    \label{fig:agentic_workflow}
\end{figure}


Figure~\ref{fig:agentic_workflow} presents the agent-based implementation view of CitySTAR. 
While the main paper describes CitySTAR as a three-stage structured reasoning pipeline (Figure~\ref{fig:citystar}), the supplementary material further explains how this pipeline is realized through collaborative functional agents. 
Each agent maintains or transforms a specific intermediate representation, including instance tokens, query cues, tool-use plans, hypergraphs, and verification feedback. 
This role-based design makes the grounding process modular and traceable: early agents prepare the query-ready scene and executable retrieval signals, intermediate agents conduct topology-centered verification, and the final agent performs cross-modal grounding with decision.

\begin{itemize}
    \item \textbf{Scene Builder} (\S\ref{sec:state_cue}) constructs the query-ready world state by converting the raw urban point cloud into open-vocabulary instance tokens with semantic, geometric, and relational information.

    \item \textbf{Query Analyst} (\S\ref{sec:state_cue}) organizes the input instruction into actionable grounding cues, including category cues, attribute cues, and spatial relation cues.

    \item \textbf{CodeLLM Orchestrator} (\S\ref{sec:codellm_orchestrator}) translates these cues into a dynamic tool-use plan, selects 2D, 3D, and spatial tools, and grounds multimodal evidence onto instance tokens to generate coarse proposals.

    \item \textbf{Query Planner} (\S\ref{sec:topology_alignment}) shifts the refinement objective from semantic matching to topology verification and determines the target-context relations to be checked.

    \item \textbf{Text Parser} (\S\ref{sec:paired_hypergraph}) converts the natural-language description into a text-side hypergraph that explicitly represents target entities, contextual objects, and relational predicates.

    \item \textbf{Instance Parser} (\S\ref{sec:paired_hypergraph}) constructs a candidate-side local hypergraph around each proposal, using only the entities and relation types relevant to the current query.

    \item \textbf{Topology Verifier} (\S\ref{sec:topology_verifier}) matches the text-side and candidate-side hypergraphs and applies bidirectional topology checking to remove candidates with unstable or reversed target-context relations.

    \item \textbf{Cross-Modal Arbiter} (\S\ref{sec:cross_modal_grounding}) verifies structurally plausible candidates with candidate-centered 2D visual evidence and combines it with topology consistency for the final decision.
\end{itemize}




\subsection{Detailed Method}
\label{sec:supp_method}

This section provides additional details of CitySTAR's methodology that complement the condensed version in the main text. All formulas, node- and edge-level evidence, and query-conditioned operations are included here for reproducibility and full technical clarity.

\subsubsection{Stage 1: Query-adaptive Multimodal Candidate Grounding}
\label{sec:supp_stage1}

Stage~1 converts raw urban point clouds into a structured query-ready scene graph. The scene is first projected into geo-aware 2D views, segmented with open-vocabulary models, lifted back to 3D, and consolidated into instance-level tokens:
\begin{equation}
\mathcal{G}_{s}=\{\mathcal{I},\mathcal{A},\mathcal{R}\},
\end{equation}
where \(\mathcal{I}\) are 3D instances, \(\mathcal{A}\) semantic and geometric attributes, and \(\mathcal{R}\) spatial relations.

The query \(q\) is organized into actionable cues:
\begin{equation}
\mathcal{C}(q)=\{\mathcal{c}_{cat},\mathcal{c}_{attr},\mathcal{c}_{sp}\},
\end{equation}
with category cues, attribute cues, and spatial cues. A CodeLLM converts these into an executable tool-use plan \(\mathcal{T}(q) = \{t_1,\dots,t_M\}\). Each tool provides node- and edge-level evidence:
\begin{equation}
\mathcal{E}^{q} = 
\left\{ \big(s_m^{n}(i\mid E_m),\, s_m^{e}(i,j\mid E_m)\big)
\; \middle|\; t_m\in\mathcal{T}(q),\, i,j\in\mathcal{I} \right\}.
\end{equation}
Candidate relevance is aggregated as:
\begin{equation}
R(i\mid q)=\sum_{m=1}^{M} w_m(q)\,s_m(i\mid t_m,\mathcal{G}_{s}),
\end{equation}
yielding a high-recall candidate pool for Stage~2.

\subsubsection{Stage 2: Topology-aware Soft Graph Alignment}
\label{sec:supp_stage2}

Stage~2 shifts the focus from semantic matching to relational verification. The query is represented as a hypergraph:
\begin{equation}
\mathcal{G}^{q}=(\mathcal{V}^{q},\mathcal{R}^{q}),
\end{equation}
where nodes correspond to target and contextual entities and hyperedges encode spatial or topological relations. For candidate \(j\), a local scene-side hypergraph is constructed:
\begin{equation}
\mathcal{G}^{s}_j=(\mathcal{V}^{s}_j,\mathcal{E}^{s}_j),
\end{equation}
restricted to the relation types in \(\mathcal{G}^{q}\). Node correspondences are established using Stage~1 evidence. Relations are verified with their inverse predicates to compute bidirectional consistency \(s_{\mathrm{bi}}(e)\). The candidate topology score is:
\begin{equation}
\mathrm{Score}_{\mathrm{topo}}(\mathcal{G}^{q},\mathcal{G}^{s}_{j}) = \frac{1}{|\mathcal{R}^{q}|} \sum_{e\in\mathcal{R}^{q}} s_{\mathrm{bi}}(e)
\end{equation}
filtering out candidates that are semantically plausible but structurally inconsistent.

\subsubsection{Stage 3: Candidate-centered 2D Visual Verification}
\label{sec:supp_stage3}

Remaining candidates are verified in the 2D visual space. For each candidate \(j\), a candidate-centered rendering is compared with the query using a visual-text reranker~\citep{zhang2025qwen3embeddingadvancingtext}, producing a visual score \(S_{\mathrm{vis}}(j)\). The final grounded instance is selected by:
\begin{equation}
j^{*} = 
\arg\max_{j} 
\Big(
\mathrm{Score}_{\mathrm{topo}}(\mathcal{G}^{q},\mathcal{G}^{s}_{j})
+
\lambda_{\mathrm{2D}} S_{\mathrm{vis}}(j)
\Big),
\end{equation}
where \(\lambda_{\mathrm{2D}}\) balances the visual contribution. This stage preserves interpretability while using cross-modal evidence to improve the final grounding decision.


% \subsection{CitySTAR-3D Dataset Construction and Enhancement}
% \label{app:dataset_enhancement}

% CitySTAR-3D is designed to evaluate reasoning-oriented city-scale 3D grounding. Compared with CityRefer and CityAnchor, it extends both semantic coverage and annotation quality while providing more complex textual descriptions for relational reasoning.

% \textbf{Data Sources and Composition.} The benchmark is built upon SensatUrban and STPLS3D. The dataset contains 1286 text-object pairs, including 686 samples from SensatUrban and 600 samples from STPLS3D. Instances are grouped into 15 semantic categories, covering general urban objects, functional buildings, vehicle-related objects, parking areas, vegetation, pedestrian paths, rail, and water infrastructure. This diversity ensures that models are evaluated on both common and functionally distinct entities.

% \textbf{Data Construction.} For each category, ground-truth instances are initially generated using 3D geometric priors. Candidate bounding boxes are constructed from raw point clouds based on object-to-object distances, object extents, and alignment with real 3D scene geometry. These initial boxes encode 3D spatial information, which helps preserve object completeness and consistency in densely structured urban scenes.

% \textbf{Annotation Refinement.} The preliminary 3D boxes are further refined using visual-language model (VLM) feedback. VLMs provide guidance for attributes such as color, texture, and contextual alignment with nearby entities, ensuring that the final annotations are consistent with both 3D geometry and textual description. After automated refinement, all annotations undergo manual verification to correct potential errors, remove duplicates, and ensure accurate bounding-box coverage.

% \textbf{Language Descriptions.} Each instance is associated with a natural-language description designed to support relational reasoning. Descriptions include containment relations, neighbor relations, attribute-based descriptions, and spatial-layout cues, requiring models to reason over object composition, adjacency, relative directions, and complex spatial configurations.

% \textbf{Summary of Advantages.} CitySTAR-3D combines open-vocabulary semantics, precise 3D geometric priors, VLM-based refinement, and human verification. The resulting benchmark provides a reliable, challenging, and diverse testbed for evaluating city-scale 3D grounding models that must understand both object-level attributes and multi-entity relational structure.relations, complex spatial layouts, and open-vocabulary entity categories.



% \begin{table*}[h]
% \centering
% \caption{Unified comparison of CityRefer, CityAnchor, and CitySTAR-3D. Orange cells highlight the enhanced capabilities of CitySTAR-3D.}
% \label{tab:unified_dataset_comparison}
% \renewcommand{\arraystretch}{1.08}
% \setlength{\tabcolsep}{4pt}
% \footnotesize
% \resizebox{\linewidth}{!}{
% \begin{tabular}{
% p{2.7cm}
% p{3.4cm}
% p{3.6cm}
% >{\columncolor{orange!16}}p{5.6cm}
% p{4.2cm}
% }
% \toprule
% \rowcolor{gray!18}
% \textbf{Aspect} 
% & \textbf{CityRefer} 
% & \textbf{CityAnchor} 
% & \textbf{CitySTAR-3D} 
% & \textbf{Significance} \\
% \midrule

% \rowcolor{gray!10}
% \multicolumn{5}{l}{\textbf{Basic Dataset Information}} \\

% Source data 
% & SensatUrban 
% & STPLS3D 
% & SensatUrban and STPLS3D 
% & Provides complementary urban scenes for evaluating city-scale grounding. \\

% Evaluation scale 
% & Over 1,000 validation queries 
% & Over 200 validation queries 
% & 1,286 text-object pairs 
% & Supports evaluation under more diverse semantic and relational settings. \\

% Data composition 
% & SensatUrban validation split 
% & STPLS3D validation split 
% & 686 samples from SensatUrban and 600 samples from STPLS3D 
% & Combines real city-scale scenes from different sources. \\

% Semantic setting 
% & 4 coarse categories 
% & 9 urban object categories 
% & 15 semantic groups 
% & Expands grounding from closed coarse labels to richer urban semantics. \\

% \midrule
% \rowcolor{gray!10}
% \multicolumn{5}{l}{\textbf{Semantic Scope}} \\

% Core urban objects 
% & Building, car, ground, parking 
% & Building, vegetation, aircraft, truck, vehicle, light pole, fence, street sign, bike 
% & Buildings, vehicles, parking areas, vegetation, pedestrian paths, rail, and water infrastructure 
% & Extends the evaluation scope beyond basic object classes. \\

% Functional building categories 
% & Not available 
% & Limited 
% & Residential, office, commercial, educational, hospitality, industrial, religious, warehouse, civic, and generic buildings 
% & Enables grounding based on urban function rather than only appearance. \\

% Relation-aware categories 
% & Limited 
% & Moderate 
% & Containment, neighbor, attribute, and spatial-layout descriptions 
% & Better evaluates compositional reasoning over target-context relations. \\

% \midrule
% \rowcolor{gray!10}
% \multicolumn{5}{l}{\textbf{Annotation Properties}} \\

% Instance annotation quality 
% & Standard object boxes 
% & Standard object boxes 
% & Refined boxes with more complete object extents 
% & Improves localization reliability and reduces box-level ambiguity. \\

% Description complexity 
% & Simple object or landmark references 
% & Object prompts with simple spatial context 
% & Attribute, containment, neighbor, and relation-aware descriptions 
% & Better evaluates compositional reasoning over multiple urban entities. \\

% Representative examples 
% & \textit{car near building} 
% & \textit{building beside tree} 
% & \textit{warehouse adjacent to parked cars and west of a river} 
% & Highlights the need for attribute, context, and relation understanding. \\

% \bottomrule
% \end{tabular}
% }
% \end{table*}
\subsection{CitySTAR-3D Dataset Construction and Enhancement}
\label{app:dataset_enhancement}

CitySTAR-3D is a reasoning-oriented city-scale 3D grounding benchmark that extends existing datasets with richer semantics, improved instance completeness, and more complex relational language descriptions.

\textbf{Data Sources and Composition.} The dataset is built upon SensatUrban and STPLS3D. It contains 1286 text-object pairs, including 686 samples from SensatUrban and 600 samples from STPLS3D. Instances are organized into 15 semantic groups covering general urban objects, functional buildings, vehicle-related objects, parking areas, vegetation, pedestrian paths, and rail or water infrastructure. This semantic diversity enables evaluation across both common and specialized urban entities.

\textbf{Data Construction.} Ground-truth instances are initially generated using 3D geometric priors. Candidate bounding boxes are derived from raw point clouds based on object-to-object distances, object extents, and real 3D scene geometry. For STPLS3D-derived samples, CitySTAR-3D adopts the same instance bounding boxes as CityAnchor but upgrades the textual descriptions to provide more relational and attribute information. 

\textbf{Annotation Refinement.} Initial 3D boxes are further refined using visual-language model (VLM) feedback to ensure consistency between visual appearance, geometry, and textual description. The refinement addresses attributes, relative positions, and neighborhood relationships. After automated refinement, all annotations undergo manual verification to correct errors, remove duplicates, and ensure complete object coverage.

\textbf{Language Descriptions.} Each instance is associated with a natural-language description that supports relation-aware grounding. Descriptions include containment, adjacency, relative directions, and spatial-layout cues, requiring models to reason over object composition and multi-entity relations.

\textbf{Summary of Advantages.} CitySTAR-3D integrates open-vocabulary semantics, 3D geometric priors, VLM refinement, and human verification. The benchmark provides a reliable, challenging, and diverse testbed for evaluating city-scale 3D grounding models. Table~\ref{tab:unified_dataset_comparison} summarizes the differences between CityRefer, CityAnchor, and CitySTAR-3D, highlighting the enhanced semantic and relational complexity. Figures~\ref{fig:CitySTAR3D-CityRefer} and~\ref{fig:CitySTAR3D-CityAnchor} visually illustrate the differences between CitySTAR-3D and the previous datasets.

\begin{table*}[h]
\centering
\caption{Unified comparison of CityRefer dataset, CityAnchor dataset, and CitySTAR-3D dataset. Orange cells highlight the enhanced capabilities of CitySTAR-3D.}
\label{tab:unified_dataset_comparison}
\renewcommand{\arraystretch}{1.08}
\setlength{\tabcolsep}{4pt}
\footnotesize
\resizebox{\linewidth}{!}{
\begin{tabular}{
p{2.7cm}
p{3.4cm}
p{3.6cm}
>{\columncolor{orange!16}}p{5.6cm}
p{4.2cm}
}
\toprule
\rowcolor{gray!18}
\textbf{Aspect} 
& \textbf{CityRefer Dataset} 
& \textbf{CityAnchor Dataset} 
& \textbf{CitySTAR-3D Dataset} 
& \textbf{Significance} \\
\midrule

\rowcolor{gray!10}
\multicolumn{5}{l}{\textbf{Basic Dataset Information}} \\

Source data 
& SensatUrban 
& STPLS3D 
& SensatUrban and STPLS3D 
& Provides complementary urban scenes for evaluating city-scale grounding. \\

Evaluation scale 
& Over 1,000 validation queries 
& Over 200 validation queries 
& 1,286 text-object pairs 
& Supports evaluation under more diverse semantic and relational settings. \\

Data composition 
& SensatUrban validation split 
& STPLS3D validation split 
& 686 samples from SensatUrban and 600 samples from STPLS3D 
& Combines real city-scale scenes from different sources. \\

Semantic setting 
& 4 coarse categories 
& 9 urban object categories 
& 15 semantic groups 
& Expands grounding from closed coarse labels to richer urban semantics. \\

\midrule
\rowcolor{gray!10}
\multicolumn{5}{l}{\textbf{Semantic Scope}} \\

Core urban objects 
& Building, car, ground, parking 
& Building, vegetation, aircraft, truck, vehicle, light pole, fence, street sign, bike 
& Buildings, vehicles, parking areas, vegetation, pedestrian paths, rail, and water infrastructure 
& Extends the evaluation scope beyond basic object classes. \\

Functional building categories 
& Not available 
& Limited 
& Residential, office, commercial, educational, hospitality, industrial, religious, warehouse, civic, and generic buildings 
& Enables grounding based on urban function rather than only appearance. \\

Relation-aware categories 
& Limited 
& Moderate 
& Containment, neighbor, attribute, and spatial-layout descriptions 
& Better evaluates compositional reasoning over target-context relations. \\

\midrule
\rowcolor{gray!10}
\multicolumn{5}{l}{\textbf{Annotation Properties}} \\

Instance annotation quality 
& Standard object boxes 
& Standard object boxes 
& Refined boxes with more complete object extents 
& Improves localization reliability and reduces box-level ambiguity. \\

Description complexity 
& Simple object or landmark references 
& Object prompts with simple spatial context 
& Attribute, containment, neighbor, and relation-aware descriptions 
& Better evaluates compositional reasoning over multiple urban entities. \\

Representative examples 
& \textit{car near building} 
& \textit{building beside tree} 
& \textit{warehouse adjacent to parked cars and west of a river} 
& Highlights the need for attribute, context, and relation understanding. \\

\bottomrule
\end{tabular}
}
\end{table*}

\begin{figure}[h]
    \centering
    \includegraphics[width=0.85\linewidth]{Figs/CitySTAR3D.jpg}
    \caption{Comparison between CitySTAR-3D dataset and CityRefer dataset. CitySTAR-3D provides richer semantic categories, more complete instance annotations, and relation-aware descriptions.}
    \label{fig:CitySTAR3D-CityRefer}
\end{figure}

\begin{figure}[h]
    \centering
    \includegraphics[width=0.85\linewidth]{Figs/CitySTAR3D_anchor.jpg}
    \caption{Comparison between CitySTAR-3D dataset and CityAnchor dataset. CitySTAR-3D uses the same bounding boxes as CityAnchor for STPLS3D samples but upgrades textual descriptions with richer relational and attribute information.}
    \label{fig:CitySTAR3D-CityAnchor}
\end{figure}



% \begin{table}[h]
% \centering
% \caption{Semantic groups covered by CitySTAR-3D.}
% \label{tab:citystar3d_semantic_groups}
% \scriptsize
% \setlength{\tabcolsep}{4pt}
% \renewcommand{\arraystretch}{0.95}
% \resizebox{\linewidth}{!}{
% \begin{tabular}{ll}
% \toprule
% \textbf{Group Type} & \textbf{Semantic Groups} \\
% \midrule
% Building functions 
% & Generic, residential, office, commercial, educational, hospitality, industrial, religious, warehouse, civic \\
% Transportation and parking 
% & Vehicle, parking / vehicle storage, pedestrian path / pavement \\
% Urban environment 
% & Vegetation / greenery, rail / water infrastructure \\
% \bottomrule
% \end{tabular}
% }
% \end{table}



% \begin{table*}[h]
% \centering
% \caption{Unified comparison of CityRefer, CityAnchor, and the enhanced CitySTAR-3D dataset. Orange cells highlight the enhanced capabilities of CitySTAR-3D.}
% \label{tab:unified_dataset_comparison}
% \renewcommand{\arraystretch}{1.18}
% \setlength{\tabcolsep}{4pt}
% \footnotesize
% \resizebox{\linewidth}{!}{
% \begin{tabular}{
% p{2.7cm}
% p{3.4cm}
% p{3.6cm}
% >{\columncolor{orange!18}}p{5.7cm}
% p{4.0cm}
% }
% \toprule
% \rowcolor{gray!18}
% \textbf{Aspect} 
% & \textbf{CityRefer} 
% & \textbf{CityAnchor} 
% & \textbf{CitySTAR-3D} 
% & \textbf{Significance} \\
% \midrule

% \rowcolor{gray!10}
% \multicolumn{5}{l}{\textbf{Basic Dataset Information}} \\

% Source data 
% & SensatUrban 
% & STPLS3D 
% & Multiple city-scale 3D scenes 
% & Broader scene coverage improves dataset diversity and generalization. \\

% Annotation scale 
% & $>35$k descriptions; $>5$k landmarks 
% & 1,448 text-object pairs 
% & --
% & Reflects the scale of grounding supervision. \\

% Category setting 
% & 4 coarse categories 
% & 9 coarse categories 
% & $>30$ high-level semantic groups with fine-grained subtypes 
% & A larger semantic space supports more challenging grounding queries. \\

% \midrule
% \rowcolor{gray!10}
% \multicolumn{5}{l}{\textbf{Semantic Scope}} \\

% Core urban objects 
% & Building, car, ground, parking 
% & Building, vegetation, aircraft, truck, vehicle, light pole, fence, street sign, bike 
% & Generic objects, vehicles, parking areas, vegetation, and pedestrian-related structures 
% & Extends coverage from basic objects to richer urban scene components. \\

% Functional building categories 
% & Not available 
% & Not available 
% & Residential, office, commercial, education, hospitality, industrial, religious, warehouse, and civic facilities 
% & Enables grounding based on urban function rather than only object appearance. \\

% Fine-grained vehicle subtypes 
% & Car only 
% & Vehicle, truck, bike, aircraft 
% & Car, SUV, van, truck, bus, motorcycle, bicycle, emergency vehicle, and service vehicle 
% & Supports fine-grained target discrimination in urban traffic scenes. \\

% Public infrastructure and environment 
% & Ground and parking only 
% & Light pole, fence, street sign, vegetation 
% & Sidewalk, crosswalk, pedestrian path, plaza, rail-related objects, river, canal, pond, and water body 
% & Provides richer contextual cues for compositional grounding. \\

% \midrule
% \rowcolor{gray!10}
% \multicolumn{5}{l}{\textbf{Annotation Properties}} \\

% Fine-grained subtype labels 
% & Limited 
% & Limited 
% & Available for vehicles, buildings, pedestrian facilities, infrastructure, and environmental objects 
% & Reduces semantic ambiguity among visually or functionally similar objects. \\

% Relation-aware descriptions 
% & Basic object-level descriptions 
% & Moderate text-object descriptions 
% & Designed for compositional and relation-aware grounding with contextual entities 
% & Better evaluates structured reasoning over multiple urban entities. \\

% Instance annotation quality 
% & Standard object annotations 
% & Standard object annotations 
% & Refined object boxes and enhanced instance semantics 
% & Improves localization precision and evaluation reliability. \\

% Representative semantic examples 
% & Building, car, parking lot 
% & Vehicle, fence, light pole, bike 
% & Apartment building, office tower, SUV, bus, sidewalk, crosswalk, warehouse, river 
% & Highlights the broader and more realistic semantic scope of CitySTAR-3D. \\

% \bottomrule
% \end{tabular}
% }
% \end{table*}



% As summarized in Table~\ref{tab:unified_dataset_comparison}, CitySTAR-3D provides a more detailed benchmark than previous city-scale grounding datasets. The improvement is not limited to a larger number of categories. More importantly, the dataset introduces functional building labels, fine-grained object subtypes, and richer contextual descriptions. These additions make the grounding task closer to real urban understanding, where a target may be identified by its category, function, appearance, neighboring objects, or spatial relation. Therefore, CitySTAR-3D is better suited for evaluating fine-grained and relation-aware grounding in complex city-scale scenes.



% \begin{figure}[h]
%     \centering
%     \includegraphics[width=0.9\linewidth]{Figs/CitySTAR3D.jpg}
%     \caption{The comparison between CitySTAR3D and CityRefer.}
%     \label{fig:CitySTAR3D-CityRefer}
% \end{figure}





% \begin{figure}[h]
%     \centering
%     \includegraphics[width=0.9\linewidth]{Figs/CitySTAR3D_anchor.jpg}
%     \caption{The comparison between CitySTAR3D and CiyAnchor.}
%     \label{fig:CitySTAR3D-CityAnchor}
% \end{figure}





\subsection{More Detailed Ablation Study}
\label{app:d_ablation_study}
\begin{table}[h]
  \centering
  \caption{Performance comparison under different candidate truncation settings.}
  \label{tab:method_comparison_v2}
  \scriptsize % 字体更小
  \renewcommand{\arraystretch}{0.7} % 更紧凑行距
  \setlength{\tabcolsep}{4pt} % 缩小列间距
  \resizebox{\linewidth}{!}{%
  \begin{tabular}{lccccc}
    \toprule
    \rowcolor{gray!15}
    \textbf{Method} 
    & \textbf{Avg. Cand.} 
    & \multicolumn{3}{c}{\textbf{Accuracy (\%)}} 
    & \textbf{Time (s)} \\
    \cmidrule(lr){3-5}
    \rowcolor{gray!15}
    & 
    & \textbf{Top-1} 
    & \textbf{Top-5} 
    & \textbf{Top-10} 
    & \\
    \midrule

    CityRefer 
    & -- 
    & 7.47 
    & 12.19 
    & 17.27 
    & 42.27 \\

    \rowcolor{gray!8}
    CityAnchor (ROI=0.35) 
    & 30.3 
    & 26.80 
    & 32.36 
    & 35.10 
    & 27.05 \\

    \rowcolor{gray!8}
    CityAnchor (ROI=0.30) 
    & 41.5 
    & 46.86 
    & 59.83 
    & 64.66 
    & 32.45 \\

    \midrule

    Ours (no truncation) 
    & 22.4 
    & 64.66 
    & 72.54 
    & 88.08 
    & 28.59 \\

    \rowcolor{orange!8}
    Ours (top-15) 
    & 13.7 
    & 69.43 
    & 74.44 
    & 86.36 
    & 24.26 \\

    \rowcolor{orange!18}
    \textbf{Ours (top-10)} 
    & \textbf{8.5} 
    & \textbf{71.68} 
    & \textbf{75.99} 
    & \textbf{85.83}
    & \underline{20.73} \\
    Ours (rule-based) 
    & - 
    & 69.08 
    & 74.26 
    & 78.75 
    & \textbf{16.53} \\
    \bottomrule
  \end{tabular}%
  }
\end{table}
% We maintain consistent settings with the baseline methods. Specifically, we do not include the scene construction time in our test-time latency measurements, even though existing methods typically require over 10 minutes for this phase. Table~\ref{tab:ablation} in the main paper verifies the contribution of each core component, including CodeLLM-driven candidate grounding, topology verification, and final cross-modal verification. As a complementary ablation, Table~\ref{tab:method_comparison_v2} further analyzes the effect of the truncation size \(K\) in the candidate reranking stage. Compared with the non-truncated setting, using top-10 truncation reduces the average candidate number from 22.4 to 8.5, with a reduction of 13.9\textcolor{red}{\(\downarrow\)}, and decreases the inference time from 28.59 to 20.73, with a reduction of 7.86\textcolor{red}{\(\downarrow\)}. Meanwhile, it still maintains a high Top-10 accuracy of 85.83, only slightly lower than 88.08 without truncation. This indicates that a compact candidate set is sufficient for reliable final grounding, while substantially improving the efficiency of the reasoning pipeline. We observe that although rule-based methods are more time-efficient, the design of CodeLLM allows for dynamic stopping or modification of the candidate scope, as well as the proactive acquisition of additional information. This results in superior performance and supports the handling of more complex QA problems in the future.


We maintain the same settings as baseline methods, excluding scene construction time from test-time latency, although it typically exceeds 10 minutes for prior approaches. Table~\ref{tab:ablation} in the main paper verifies the contribution of each core component, including CodeLLM-driven candidate grounding, topology verification, and cross-modal verification. Table~\ref{tab:method_comparison_v2} further analyzes the effect of truncation size \(K\) in candidate reranking. Using top-10 truncation reduces the average candidate number from 22.4 to 8.5 (\(\downarrow 13.9\)) and decreases inference time from 28.59 to 20.73 seconds (\(\downarrow 7.86\)), while retaining a high Top-10 accuracy of 85.83, slightly lower than 88.08 without truncation. This demonstrates that a compact candidate set suffices for reliable grounding and substantially improves reasoning efficiency. CodeLLM supports dynamic candidate scope adjustment and proactive evidence acquisition, enabling higher performance and future handling of more complex QA tasks.




% \subsection{More detailed Ablation Study}
% \label{app:d_ablation_study}

% Table~\ref{tab:ablation} in the main paper verifies the contribution of each core component, including CodeLLM-driven candidate grounding, topology verification, and final cross-modal verification. As a complementary ablation, Table~\ref{tab:method_comparison_v2} further analyzes the effect of the truncation size \(K\) in the candidate reranking stage. Compared with the non-truncated setting, using top-10 truncation reduces the average candidate number from 22.4 to 8.5, with a reduction of 13.9\textcolor{red}{\(\downarrow\)}, and decreases the inference time from 28.59 to 20.73, with a reduction of 7.86\textcolor{red}{\(\downarrow\)}. Meanwhile, it still maintains a high Top-10 accuracy of 85.83, only slightly lower than 88.08 without truncation. This indicates that a compact candidate set is sufficient for reliable final grounding, while substantially improving the efficiency of the reasoning pipeline.



% \begin{table}[h]
%   \centering
%   \caption{Performance comparison with different candidate truncation settings.}
%   \label{tab:method_comparison_v2}
%   \scriptsize
%   % \setlength{\tabcolsep}{4.5pt}
%   \renewcommand{\arraystretch}{1}
  
%   \begin{tabular}{lccccc}
%     \toprule
%     \rowcolor{gray!15}
%     \textbf{Method} 
%     & \textbf{Avg. Cand.} 
%     & \multicolumn{3}{c}{\textbf{Accuracy}} 
%     & \textbf{Time} \\
%     \cmidrule(lr){3-5}
%     \rowcolor{gray!15}
%     & 
%     & \textbf{Top-1} 
%     & \textbf{Top-5} 
%     & \textbf{Top-10} 
%     & \textbf{sec.} \\
%     \midrule

%     CityRefer 
%     & -- 
%     & 7.47 
%     & 12.19 
%     & 17.27 
%     & 42.27 \\

%     \rowcolor{gray!8}
%     CityAnchor (ROI=0.35) 
%     & 30.3 
%     & 26.80 
%     & 32.36 
%     & 35.10 
%     & 27.05 \\

%     \rowcolor{gray!8}
%     CityAnchor (ROI=0.30) 
%     & 41.5 
%     & 46.86 
%     & 59.83 
%     & 64.66 
%     & 32.45 \\

%     \midrule

%     Ours (no truncation) 
%     & 22.4 
%     & 64.66 
%     & 72.54 
%     & \textbf{88.08} 
%     & 28.59 \\

%     \rowcolor{orange!8}
%     Ours (top-15) 
%     & 13.7 
%     & 69.43 
%     & 74.44 
%     & 86.36 
%     & 24.26 \\

%     \rowcolor{orange!18}
%     \textbf{Ours (top-10)} 
%     & \textbf{8.5} 
%     & \textbf{71.68} 
%     & \textbf{75.99} 
%     & 85.83 
%     & \textbf{20.73} \\

%     \bottomrule
%   \end{tabular}%
% \end{table}


\subsection{Structured Information Extraction Prompt}

To facilitate systematic extraction of objects, attributes, and spatial relations from natural-language urban scene descriptions, we designed a dedicated prompt for generating structured JSON outputs. This prompt ensures that both main and related objects are captured with open-vocabulary categories, visual and 3D attributes, landmark associations, and explicit relations. Key components include:

\begin{itemize}
    \item \textbf{Main and Related Object Identification:} The central object in a description is assigned the id \texttt{"main"}, while all other concrete objects are listed as \texttt{"object1"}, \texttt{"object2"}, etc.
    \item \textbf{Attribute Extraction:} Visual attributes (color, material, shape, visibility), fine-grained category names, and 3D/geometric properties (size, length, width, height, orientation, pose, occlusion) are captured for each object.
    \item \textbf{Relation Mapping:} Relations between the main object and others are explicitly extracted, including directional, topological, distance, functional, part-whole, semantic, visual, 3D-geometric, composite, and uncategorized types. Each relation includes subject, object, phrase, type, reference anchor, and evidence.
    \item \textbf{Landmark Integration:} Objects matching provided landmark lists are linked to standard landmark names to allow semantic grounding and evaluation.
    \item \textbf{Output Standardization:} JSON structure is strictly enforced with all fields present, using empty strings for unstated information to maintain uniformity across scenes.
\end{itemize}

\noindent An example input and output illustrate the prompt’s usage:

\textbf{Input:} "The large red brick hotel is located next to the Central House. A blue bus is parked in front of it near Fifth Avenue. The hotel is about 20 meters tall and faces east."  

\textbf{Landmark list:} \texttt{["Central House", "Fifth Avenue", "Hyde Park"]}  

\textbf{Output:} JSON capturing the main hotel, nearby buildings, vehicles, and their relations, including spatial and landmark information, as shown in the structured schema above.

This prompt serves as the backbone for our semi-automated dataset construction, enabling consistent extraction of semantic, geometric, and relational information across large-scale urban point cloud and image descriptions.

\subsection{Details of CodeLLM-driven Tool Orchestration}
\label{app:codellm_tools}

Instead of relying on pre-defined retrieval rules, we use a CodeLLM-driven formulation to organize the grounding process. This is motivated by the compositional and open-ended nature of city-scale language queries. A query may involve category, appearance, geometric attribute, landmark, region, and inter-object relation at the same time. Manually designing rules for all possible cue combinations is not only labor-intensive, but also difficult to scale to unseen expressions and new tool types. The CodeLLM therefore acts as an adaptive orchestrator: it converts the parsed query into an executable sequence of tool calls, selects the required tools according to the query semantics, and adjusts the grounding path based on intermediate evidence.

This design is particularly important for billion-scale urban point clouds, where direct matching between language embeddings and all instance-level features is neither efficient nor reliable. Due to the large candidate space and the ambiguity of feature-level similarity, purely implicit retrieval can easily return visually plausible but spatially inconsistent objects. We instead reformulate grounding as executable constraint reasoning, where natural language is translated into explicit and computable operations over the query-ready world state. As a result, the system can first reduce the search space through semantic, visual, and geometric filters, and then verify the remaining candidates with metric 3D relations. The same formulation also provides a natural interface for feedback-based refinement, since an incorrect grounding path can be diagnosed and revised by regenerating alternative tool sequences.

\begin{table*}[h]
\centering
\caption{
Tool taxonomy for multimodal grounding. Query tools perform semantic and attribute filtering, 2D tools provide visual evidence, and true 3D tools operate in metric space for spatial reasoning.
}
\label{tab:tool_taxonomy}
\scriptsize
\setlength{\tabcolsep}{4pt}
\renewcommand{\arraystretch}{1.12}
\resizebox{\linewidth}{!}{
\begin{tabular}{
p{2.3cm}
p{3.0cm}
p{4.8cm}
p{6.0cm}
}
\toprule
\rowcolor{gray!15}
\textbf{Tool Group}
& \textbf{Tool}
& \textbf{Compact Signature}
& \textbf{Role in Grounding} \\
\midrule

\rowcolor{gray!8}
\multicolumn{4}{l}{\textbf{Query-level filtering}} \\

Query 
& Semantic Query 
& \texttt{semantic\_query(q, C) $\rightarrow$ IDs}
& Selects candidate instances whose semantic labels match the query. \\

Query 
& Landmark Query 
& \texttt{locate\_object(name, S) $\rightarrow$ (ID, xyz)}
& Retrieves named landmarks and provides anchor coordinates for chained reasoning. \\

Query 
& BBox Attribute Query 
& \texttt{query\_bbox(C, attr) $\rightarrow$ (ID, value)}
& Filters objects by geometric attributes such as tallest, largest, or widest. \\

Query 
& Region Query 
& \texttt{query\_region(r, S) $\rightarrow$ IDs}
& Selects objects within map-level regions, such as a street corner or northern area. \\

\midrule
\rowcolor{gray!8}
\multicolumn{4}{l}{\textbf{2D visual evidence}} \\

2D 
& Color CLIP 
& \texttt{filter\_color(q, I, C) $\rightarrow$ (ID, score)}
& Uses image-level appearance cues, especially color and texture, to rank candidates. \\

2D 
& Visual-Context Encoding 
& \texttt{encode\_context(I, C) $\rightarrow$ (ID, score)}
& Verifies visual context and image-level spatial plausibility around each candidate. \\

\midrule
\rowcolor{orange!18}
\multicolumn{4}{l}{\textbf{True 3D metric reasoning}} \\

\rowcolor{orange!8}
True 3D 
& 3D Semantic Encoding 
& \texttt{encode\_3d(q, C) $\rightarrow$ (ID, score)}
& Computes semantic similarity using point-cloud features and 3D instance tokens. \\

\rowcolor{orange!8}
True 3D 
& Distance Filter 
& \texttt{filter\_distance(a, C) $\rightarrow$ (ID, dist)}
& Filters candidates by metric distance to an anchor object or location. \\

\rowcolor{orange!8}
True 3D 
& Inter-object Distance 
& \texttt{compute\_distance(i, j) $\rightarrow$ dist}
& Measures object-to-object distance for explicit spatial reasoning. \\

\rowcolor{orange!8}
True 3D 
& Spatial Relation 
& \texttt{check\_relation(i, j, r) $\rightarrow$ bool}
& Checks relations such as \texttt{left\_of}, \texttt{behind}, \texttt{near}, or \texttt{between}. \\

\bottomrule
\end{tabular}
}
\end{table*}

As shown in Table~\ref{tab:tool_taxonomy}, the tool library covers three levels of evidence. Query-level tools provide fast semantic, landmark, attribute, and region-based filtering; 2D tools introduce appearance and image-context evidence; and true 3D tools compute metric distances, object-to-object relations, and spatial constraints. This modular design makes the grounding process both interpretable and extensible. Beyond returning candidate instances, the same interface can be expanded to output auxiliary spatial attributes, such as object height, object-to-object distance, and relative orientation, which further support topology-aware verification and future feedback-driven reasoning.

\subsubsection{CodeLLM Example Workflow}

To illustrate how the system operates, consider the following grounding query executed by CodeLLM:

\begin{enumerate}
    \item \textbf{Semantic filtering:} Select all candidate instances labeled as \texttt{hotel} using \texttt{semantic\_query} (C1). 
    \item \textbf{Geometric selection:} Retain the largest hotel instance using \texttt{query\_bbox} (C2). 
    \item \textbf{Visual filtering:} Rank candidates by red brick appearance via \texttt{filter\_color} (C3). 
    \item \textbf{Landmark localization:} Retrieve "Central House" coordinates using \texttt{locate\_object} (A1). 
    \item \textbf{Distance-based filtering:} Keep candidates within metric proximity to the landmark using \texttt{filter\_distance} (C4). 
    \item \textbf{Relation verification:} Confirm the spatial relation "near" between the candidate and landmark using \texttt{check\_relation} (R1). 
    \item \textbf{Context encoding:} Encode visual context around the candidate with \texttt{encode\_context} (CTX1). 
    \item \textbf{Graph construction:} Assign node attributes (\texttt{color, material, size}) via \texttt{assign\_node\_attr} (G1), attach landmark anchor (\texttt{assign\_anchor}, G2), and encode verified edges (\texttt{assign\_edge}, G3).
    \item \textbf{Grounding graph assembly:} Construct the \texttt{GroundingGraph} (ANSWER) integrating nodes, edges, and contextual evidence.
\end{enumerate}

This example demonstrates how CodeLLM converts high-level natural-language queries into executable operations across semantic, visual, and metric reasoning, producing interpretable and robust open-vocabulary 3D grounding outputs.


% \subsection{Details of CodeLLM-driven Tool Orchestration}
% \label{app:codellm_tools}

% Instead of relying on pre-defined retrieval rules, we use a CodeLLM-driven formulation to organize the grounding process. This is motivated by the compositional and open-ended nature of city-scale language queries. A query may involve category, appearance, geometric attribute, landmark, region, and inter-object relation at the same time. Manually designing rules for all possible cue combinations is not only labor-intensive, but also difficult to scale to unseen expressions and new tool types. The CodeLLM therefore acts as an adaptive orchestrator: it converts the parsed query into an executable sequence of tool calls, selects the required tools according to the query semantics, and adjusts the grounding path based on intermediate evidence.

% This design is particularly important for billion-scale urban point clouds, where direct matching between language embeddings and all instance-level features is neither efficient nor reliable. Due to the large candidate space and the ambiguity of feature-level similarity, purely implicit retrieval can easily return visually plausible but spatially inconsistent objects. We instead reformulate grounding as executable constraint reasoning, where natural language is translated into explicit and computable operations over the query-ready world state. As a result, the system can first reduce the search space through semantic, visual, and geometric filters, and then verify the remaining candidates with metric 3D relations. The same formulation also provides a natural interface for feedback-based refinement, since an incorrect grounding path can be diagnosed and revised by regenerating alternative tool sequences.


% \begin{table*}[h]
% \centering
% \caption{
% Tool taxonomy for multimodal grounding. Query tools perform semantic and attribute filtering, 2D tools provide visual evidence, and true 3D tools operate in metric space for spatial reasoning.
% }
% \label{tab:tool_taxonomy}
% \scriptsize
% \setlength{\tabcolsep}{4pt}
% \renewcommand{\arraystretch}{1.12}
% \resizebox{\linewidth}{!}{
% \begin{tabular}{
% p{2.3cm}
% p{3.0cm}
% p{4.8cm}
% p{6.0cm}
% }
% \toprule
% \rowcolor{gray!15}
% \textbf{Tool Group}
% & \textbf{Tool}
% & \textbf{Compact Signature}
% & \textbf{Role in Grounding} \\
% \midrule

% \rowcolor{gray!8}
% \multicolumn{4}{l}{\textbf{Query-level filtering}} \\

% Query 
% & Semantic Query 
% & \texttt{semantic\_query(q, C) $\rightarrow$ IDs}
% & Selects candidate instances whose semantic labels match the query. \\

% Query 
% & Landmark Query 
% & \texttt{locate\_object(name, S) $\rightarrow$ (ID, xyz)}
% & Retrieves named landmarks and provides anchor coordinates for chained reasoning. \\

% Query 
% & BBox Attribute Query 
% & \texttt{query\_bbox(C, attr) $\rightarrow$ (ID, value)}
% & Filters objects by geometric attributes such as tallest, largest, or widest. \\

% Query 
% & Region Query 
% & \texttt{query\_region(r, S) $\rightarrow$ IDs}
% & Selects objects within map-level regions, such as a street corner or northern area. \\

% \midrule
% \rowcolor{gray!8}
% \multicolumn{4}{l}{\textbf{2D visual evidence}} \\

% 2D 
% & Color CLIP 
% & \texttt{filter\_color(q, I, C) $\rightarrow$ (ID, score)}
% & Uses image-level appearance cues, especially color and texture, to rank candidates. \\

% 2D 
% & Visual-Context Encoding 
% & \texttt{encode\_context(I, C) $\rightarrow$ (ID, score)}
% & Verifies visual context and image-level spatial plausibility around each candidate. \\

% \midrule
% \rowcolor{orange!18}
% \multicolumn{4}{l}{\textbf{True 3D metric reasoning}} \\

% \rowcolor{orange!8}
% True 3D 
% & 3D Semantic Encoding 
% & \texttt{encode\_3d(q, C) $\rightarrow$ (ID, score)}
% & Computes semantic similarity using point-cloud features and 3D instance tokens. \\

% \rowcolor{orange!8}
% True 3D 
% & Distance Filter 
% & \texttt{filter\_distance(a, C) $\rightarrow$ (ID, dist)}
% & Filters candidates by metric distance to an anchor object or location. \\

% \rowcolor{orange!8}
% True 3D 
% & Inter-object Distance 
% & \texttt{compute\_distance(i, j) $\rightarrow$ dist}
% & Measures object-to-object distance for explicit spatial reasoning. \\

% \rowcolor{orange!8}
% True 3D 
% & Spatial Relation 
% & \texttt{check\_relation(i, j, r) $\rightarrow$ bool}
% & Checks relations such as \texttt{left\_of}, \texttt{behind}, \texttt{near}, or \texttt{between}. \\

% \bottomrule
% \end{tabular}
% }
% \end{table*}


% As shown in Table~\ref{tab:tool_taxonomy}, the tool library covers three levels of evidence. Query-level tools provide fast semantic, landmark, attribute, and region-based filtering; 2D tools introduce appearance and image-context evidence; and true 3D tools compute metric distances, object-to-object relations, and spatial constraints. This modular design makes the grounding process both interpretable and extensible. Beyond returning candidate instances, the same interface can be expanded to output auxiliary spatial attributes, such as object height, object-to-object distance, and relative orientation, which further support topology-aware verification and future feedback-driven reasoning.




\subsection{Open-vocabulary Segmentation Analysis}
\label{app:ov_segmentation}

Figure~\ref{fig:ovseg3d} compares the 3D instance segmentation results of CityRefer, CityAnchor, and CitySTAR in the same urban region for both \textbf{car} and \textbf{building} classes. Bounding boxes from all predicted instances are visualized to highlight the candidate set quality before language-guided grounding. CityRefer generates numerous oversized car and building boxes and often activates irrelevant background regions, including roads, vegetation, and other structures. CityAnchor improves object-level coverage but still produces incomplete boxes for small or densely arranged vehicles and buildings, and occasionally misses valid instances. In contrast, CitySTAR provides more accurate and complete instance masks, producing tighter and well-aligned bounding boxes with fewer false positives. This cleaner candidate set strengthens geometric and topological evidence, facilitating better target disambiguation and relation-aware grounding.

\begin{figure}[h]
    \centering
    \includegraphics[width=0.95\linewidth]{Figs/OVSeg3d.jpg}
    \caption{Qualitative comparison of open-vocabulary 3D segmentation. CitySTAR yields more accurate and complete instance masks for cars and buildings, whereas CityRefer and CityAnchor often produce oversized, fragmented, or missing boxes. This improved segmentation directly benefits downstream relation-aware grounding.}
    \label{fig:ovseg3d}
\end{figure}




% \begin{table}[h]
%   \centering
%   \caption{Performance comparison with average candidates.}
%   \label{tab:method_comparison_v2}
%   \begin{tabular}{lccccc}
%     \toprule
%     \textbf{Method} & \textbf{Avg. Candidates} & \multicolumn{4}{c}{\textbf{acc}} \\
%     \cmidrule(lr){3-6}
%      & & \textbf{Top1} & \textbf{Top5} & \textbf{Top10} & \textbf{Times} \\
%     \midrule
%     CityRefer & - & 7.47 & 12.19 & 17.27 & 42.27 \\
%     CityAnchor (ROI=0.35) & 30.3 & 26.80 & 32.36 & 35.10 & 27.05 \\
%     CityAnchor (ROI=0.30) & 41.5 & 46.86 & 59.83 & 64.66 & 32.45 \\
%     Ours (no truncation) & 22.4 & 64.66 & 72.54 & 88.08 & 28.59 \\
%     Ours (truncation=top15) & 13.7 & 69.43 & 74.44 & 86.36 & 24.26 \\
%     Ours (truncation=top10) & 8.5 & 71.68 & 75.99 & 85.83 & 20.73 \\
%     \bottomrule
%   \end{tabular}
% \end{table}

% \subsection{Additional Grounding Results and Failure Cases}
% \label{app:additional_grounding}





% \subsection{Additional Grounding Results }
% \label{app:additional_grounding}

% Figures~\ref{fig:case1} and~\ref{fig:case2} provide additional qualitative comparisons among CityRefer, CityAnchor, and CitySTAR. These examples further show two advantages of CitySTAR. First, CitySTAR improves target selection in cluttered city-scale scenes, where many nearby objects share similar appearance or category labels. CityRefer and CityAnchor may select a visually plausible but incorrect object, especially when the query contains multiple contextual cues. CitySTAR better follows the full description and identifies the intended target by jointly considering semantic, visual, and spatial evidence. Second, CitySTAR produces more accurate bounding boxes once the target is selected. Its predictions are usually tighter and better aligned with the object extent, while the baseline results often include surrounding regions or miss part of the target. These observations are consistent with the quantitative gains reported in the main paper, suggesting that CitySTAR improves both candidate disambiguation and object-level localization.



% \begin{figure}
%     \centering
%     \includegraphics[width=1\linewidth]{Figs/Suppli_citystar.jpg}
%     \caption{Enter Caption}
%     \label{fig:placeholder}
% \end{figure}


% \begin{figure}[htbp]
%     \centering
%     \includegraphics[width=\linewidth]{Figs/Suppli_case01.jpg}
%     \caption{
%     Additional qualitative comparison on correct target selection. Each row shows the grounding result of CityRefer, CityAnchor, and CitySTAR for the same language query. CitySTAR more reliably selects the intended object in cluttered urban scenes, while the baselines may localize a nearby but incorrect target.
%     }
%     \label{fig:case1}
% \end{figure}

% \begin{figure}[htbp]
%     \centering
%     \includegraphics[width=\linewidth]{Figs/Suppli_case02.jpg}
%     \caption{
%     Additional qualitative comparison on accurate bounding box localization. CitySTAR produces tighter and better aligned boxes for the referred objects, whereas CityRefer and CityAnchor often generate loose, incomplete, or shifted boxes.
%     }
%     \label{fig:case2}
% \end{figure}

\subsection{Additional Grounding Results on CitySTAR-3D}
\label{app:additional_grounding}

Figures~\ref{fig:case1},~\ref{fig:case2}, and~\ref{fig:CitySTAR3D_results} show qualitative comparisons among CityRefer, CityAnchor, and CitySTAR. CitySTAR more reliably identifies the intended target in cluttered scenes and produces tighter, better-aligned bounding boxes. Baselines may select visually plausible but incorrect objects or generate loose/incomplete boxes. The improvements benefit from our high-fidelity open-vocabulary 3D segmentation (see Section~\ref{app:ov_segmentation}).

Figure~\ref{fig:case1} highlights correct target selection. Figure~\ref{fig:case2} illustrates bounding-box accuracy. Figure~\ref{fig:CitySTAR3D_results} shows grounding on CitySTAR3D, where CitySTAR yields more precise boxes and preserves contextual relations even when baselines correctly locate the target.

\begin{figure}[h]
    \centering
    \includegraphics[width=0.95\linewidth]{Figs/Suppli_citystar.jpg}
    \vspace{-6pt}
    \caption{Qualitative grounding examples on the CitySTAR3D benchmark. CitySTAR improves both target selection and bounding-box accuracy, benefiting from open-vocabulary 3D segmentation and relation-aware cues. Even when baselines correctly select the target, CitySTAR produces better-aligned boxes and preserves contextual relations.}
    \vspace{-6pt}
    \label{fig:CitySTAR3D_results}
\end{figure}

\begin{figure}[htbp]
    \centering
    
    \includegraphics[width=\linewidth]{Figs/Suppli_case01.jpg}
    \vspace{-6pt}
    \caption{Additional qualitative comparison on correct target selection. Each row shows the grounding results of CityRefer, CityAnchor, and CitySTAR for the same language query. CitySTAR more reliably identifies the intended target in cluttered urban scenes.}
    \vspace{-6pt}
    \label{fig:case1}
\end{figure}

\begin{figure}[htbp]
    \centering
    \includegraphics[width=\linewidth]{Figs/Suppli_case02.jpg}
    \caption{Additional qualitative comparison on bounding-box localization. CitySTAR produces tighter and more accurate boxes for the referred objects, while CityRefer and CityAnchor often generate loose or incomplete boxes.}
    \label{fig:case2}
\end{figure}
